# Supplementary material for: Lang3DSG: Language-based contrastive pre-training for 3D Scene Graph prediction
Source: arXiv:2310.16494 source file (2023-10-25)

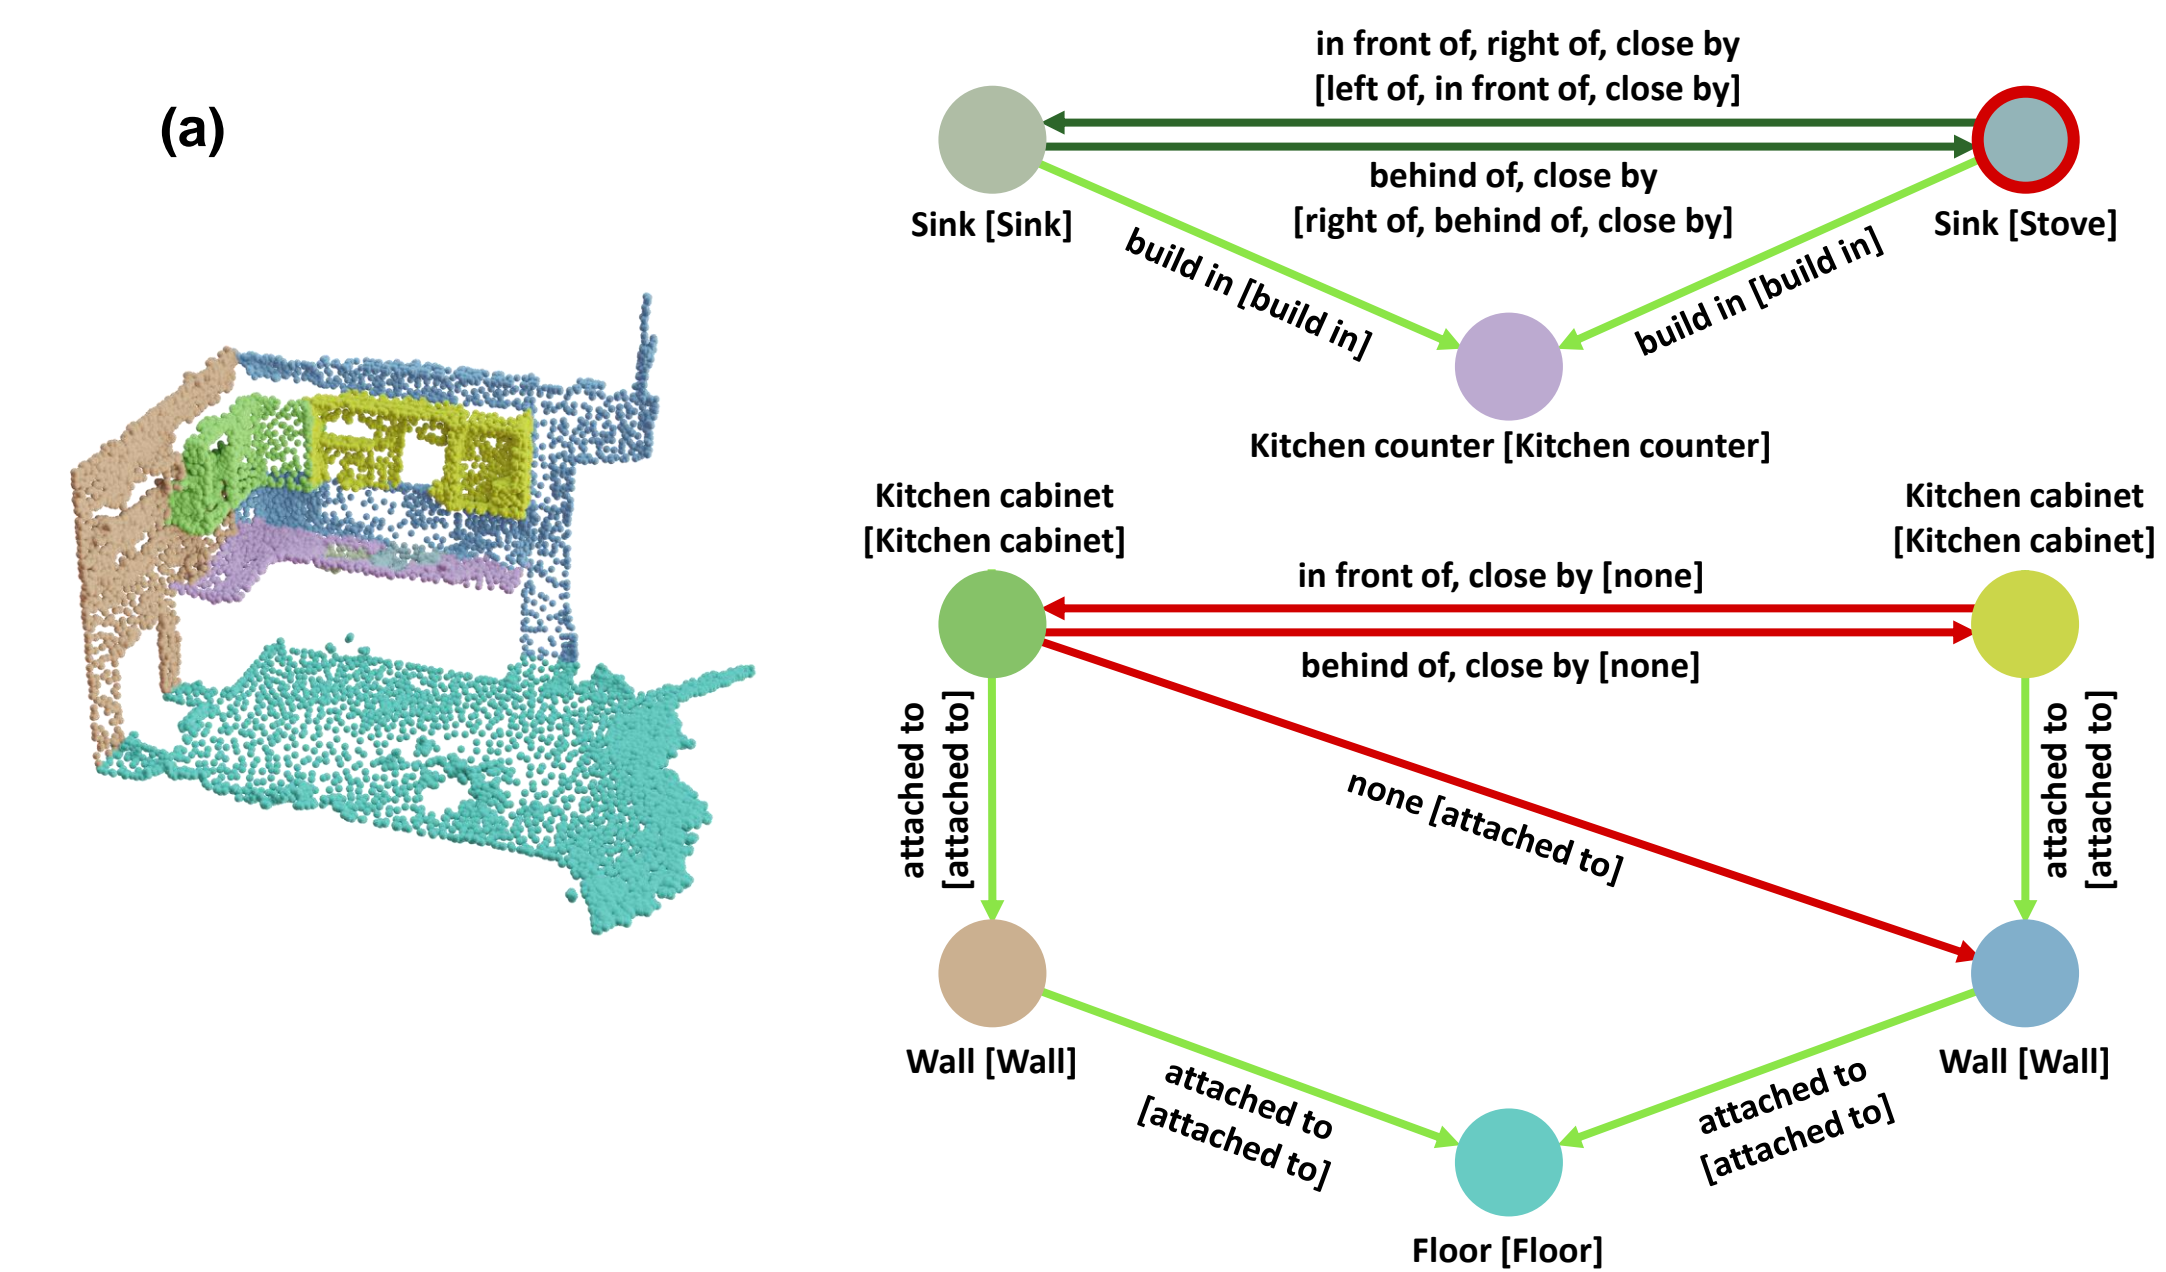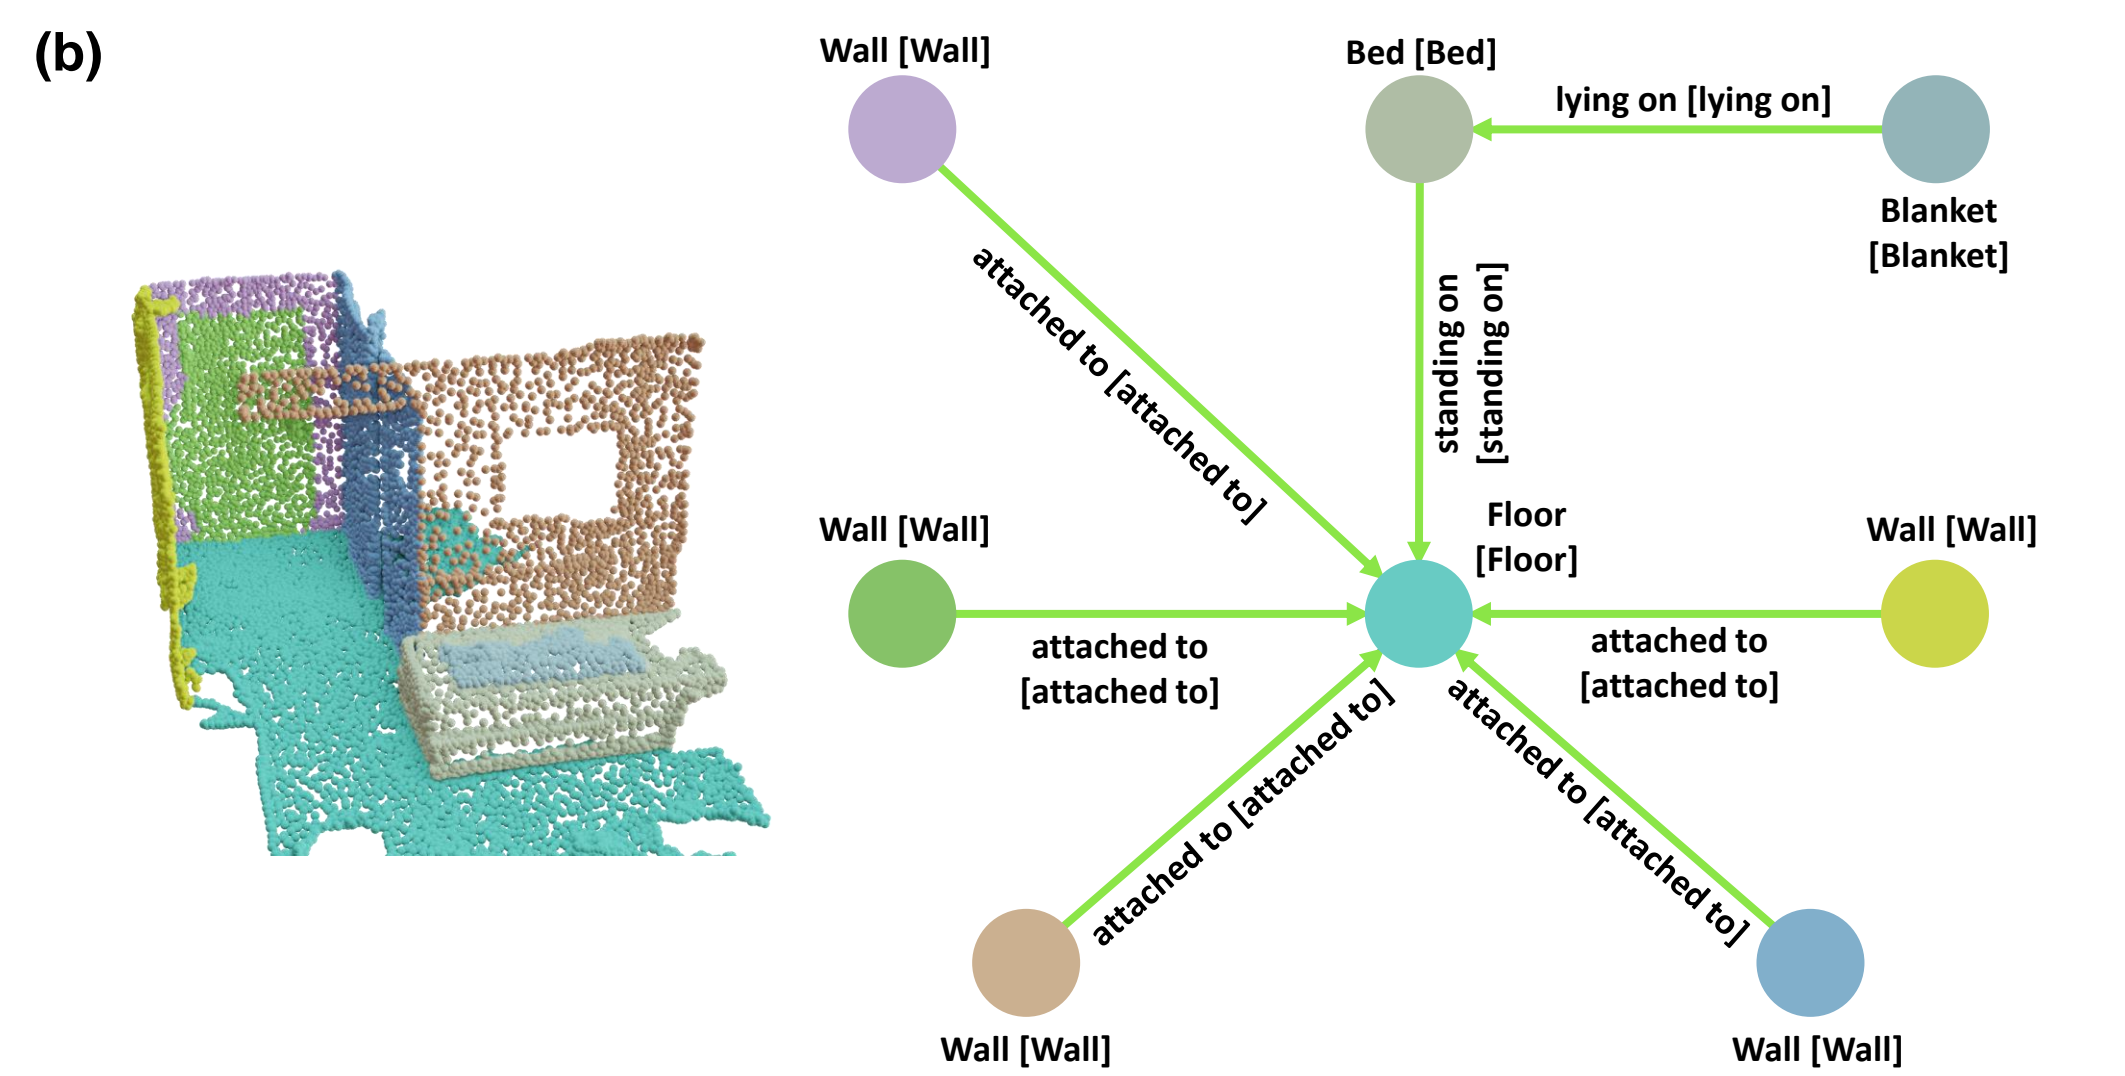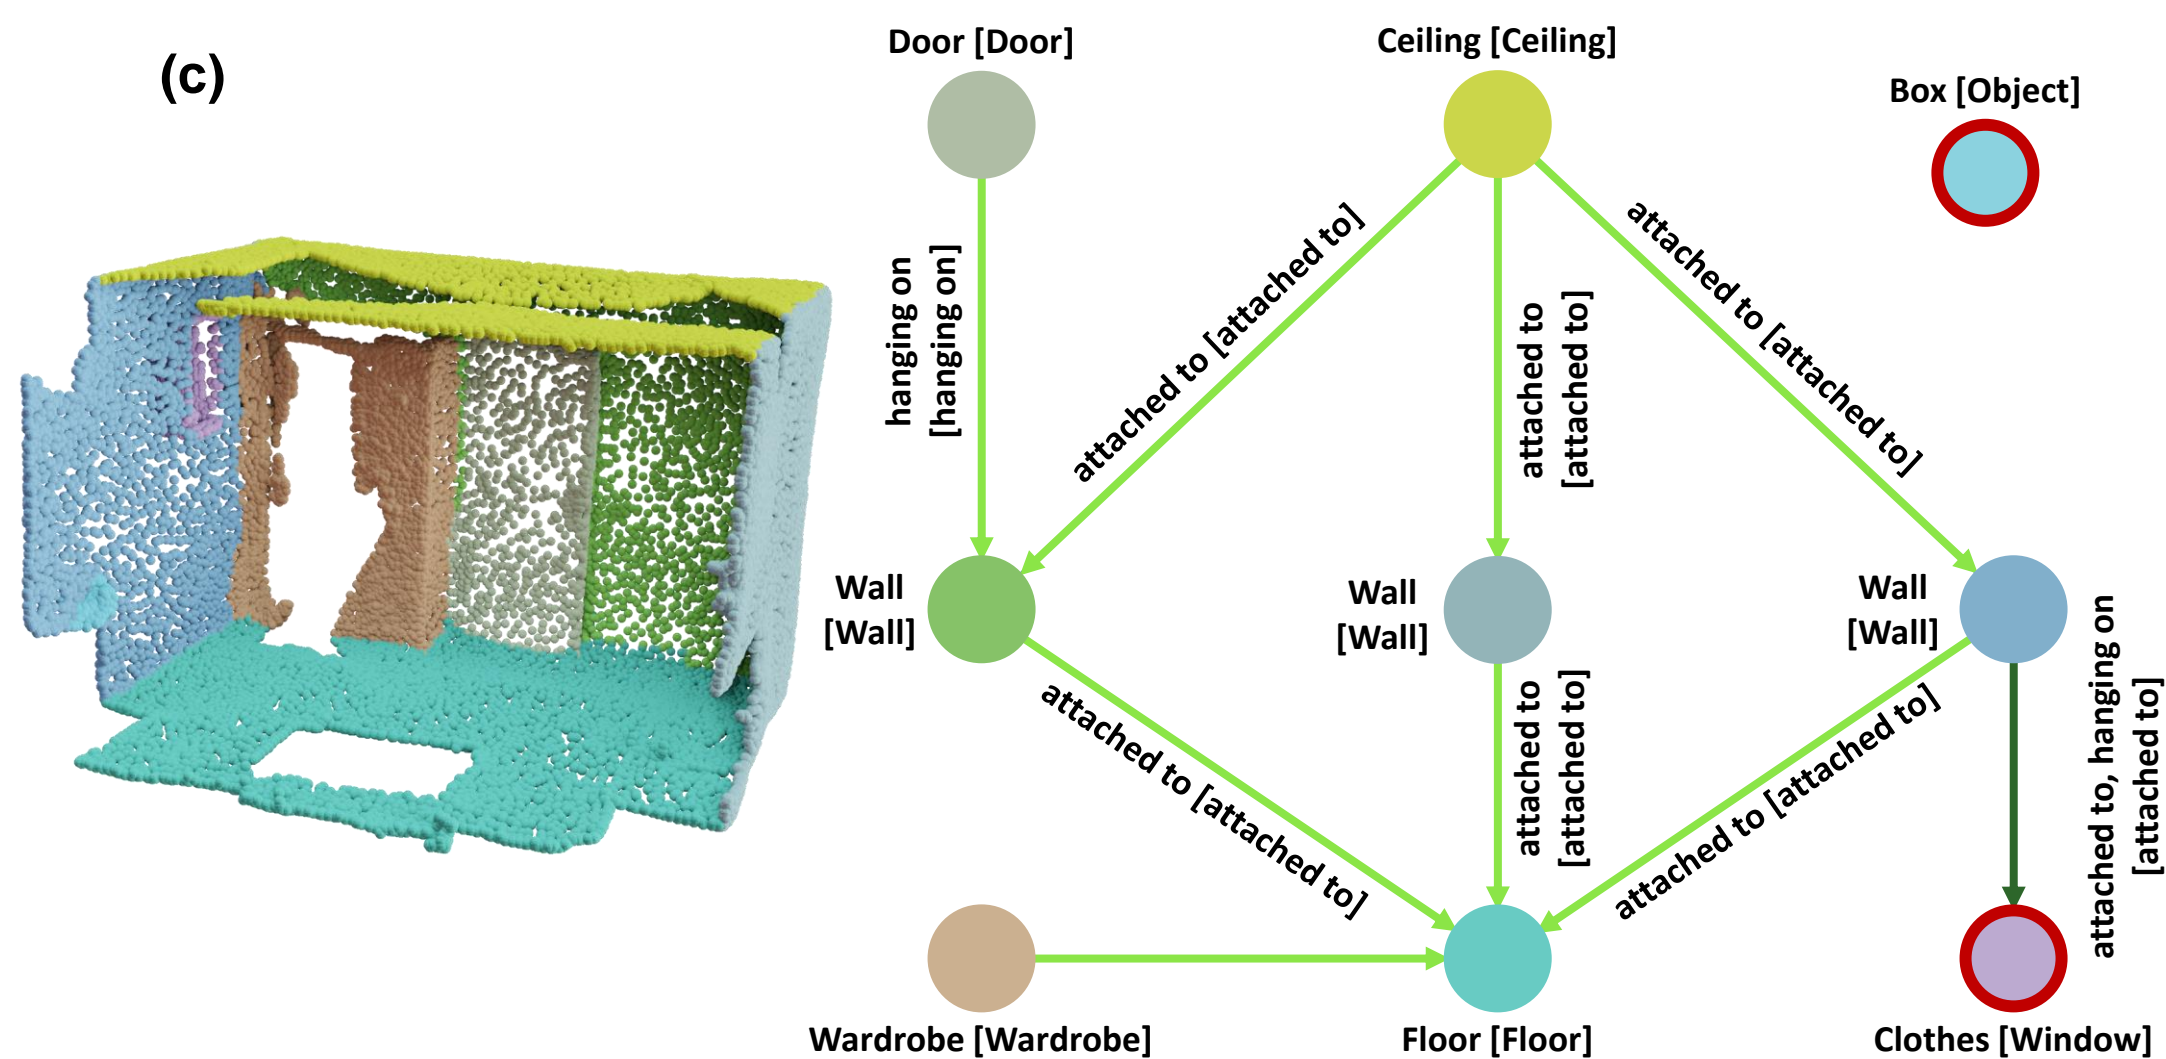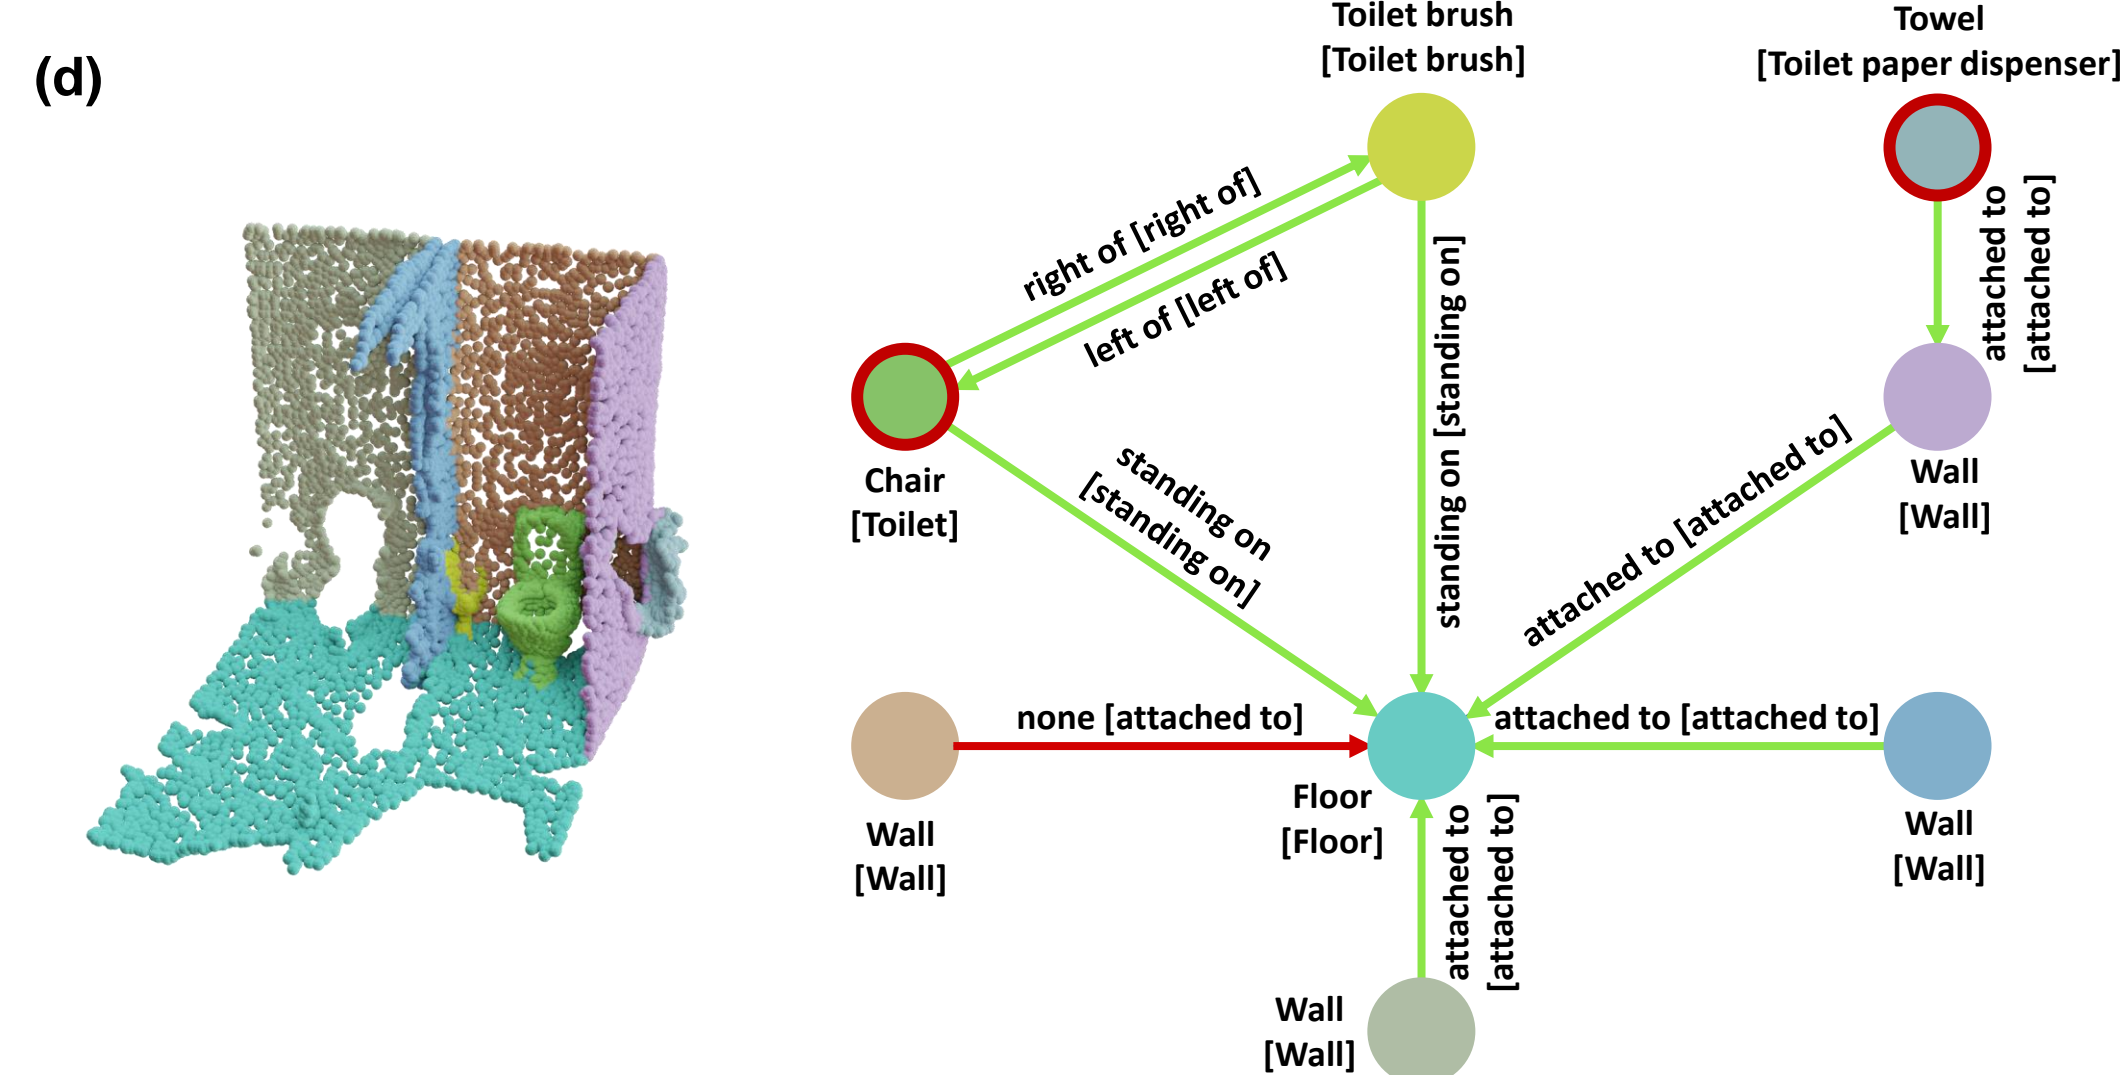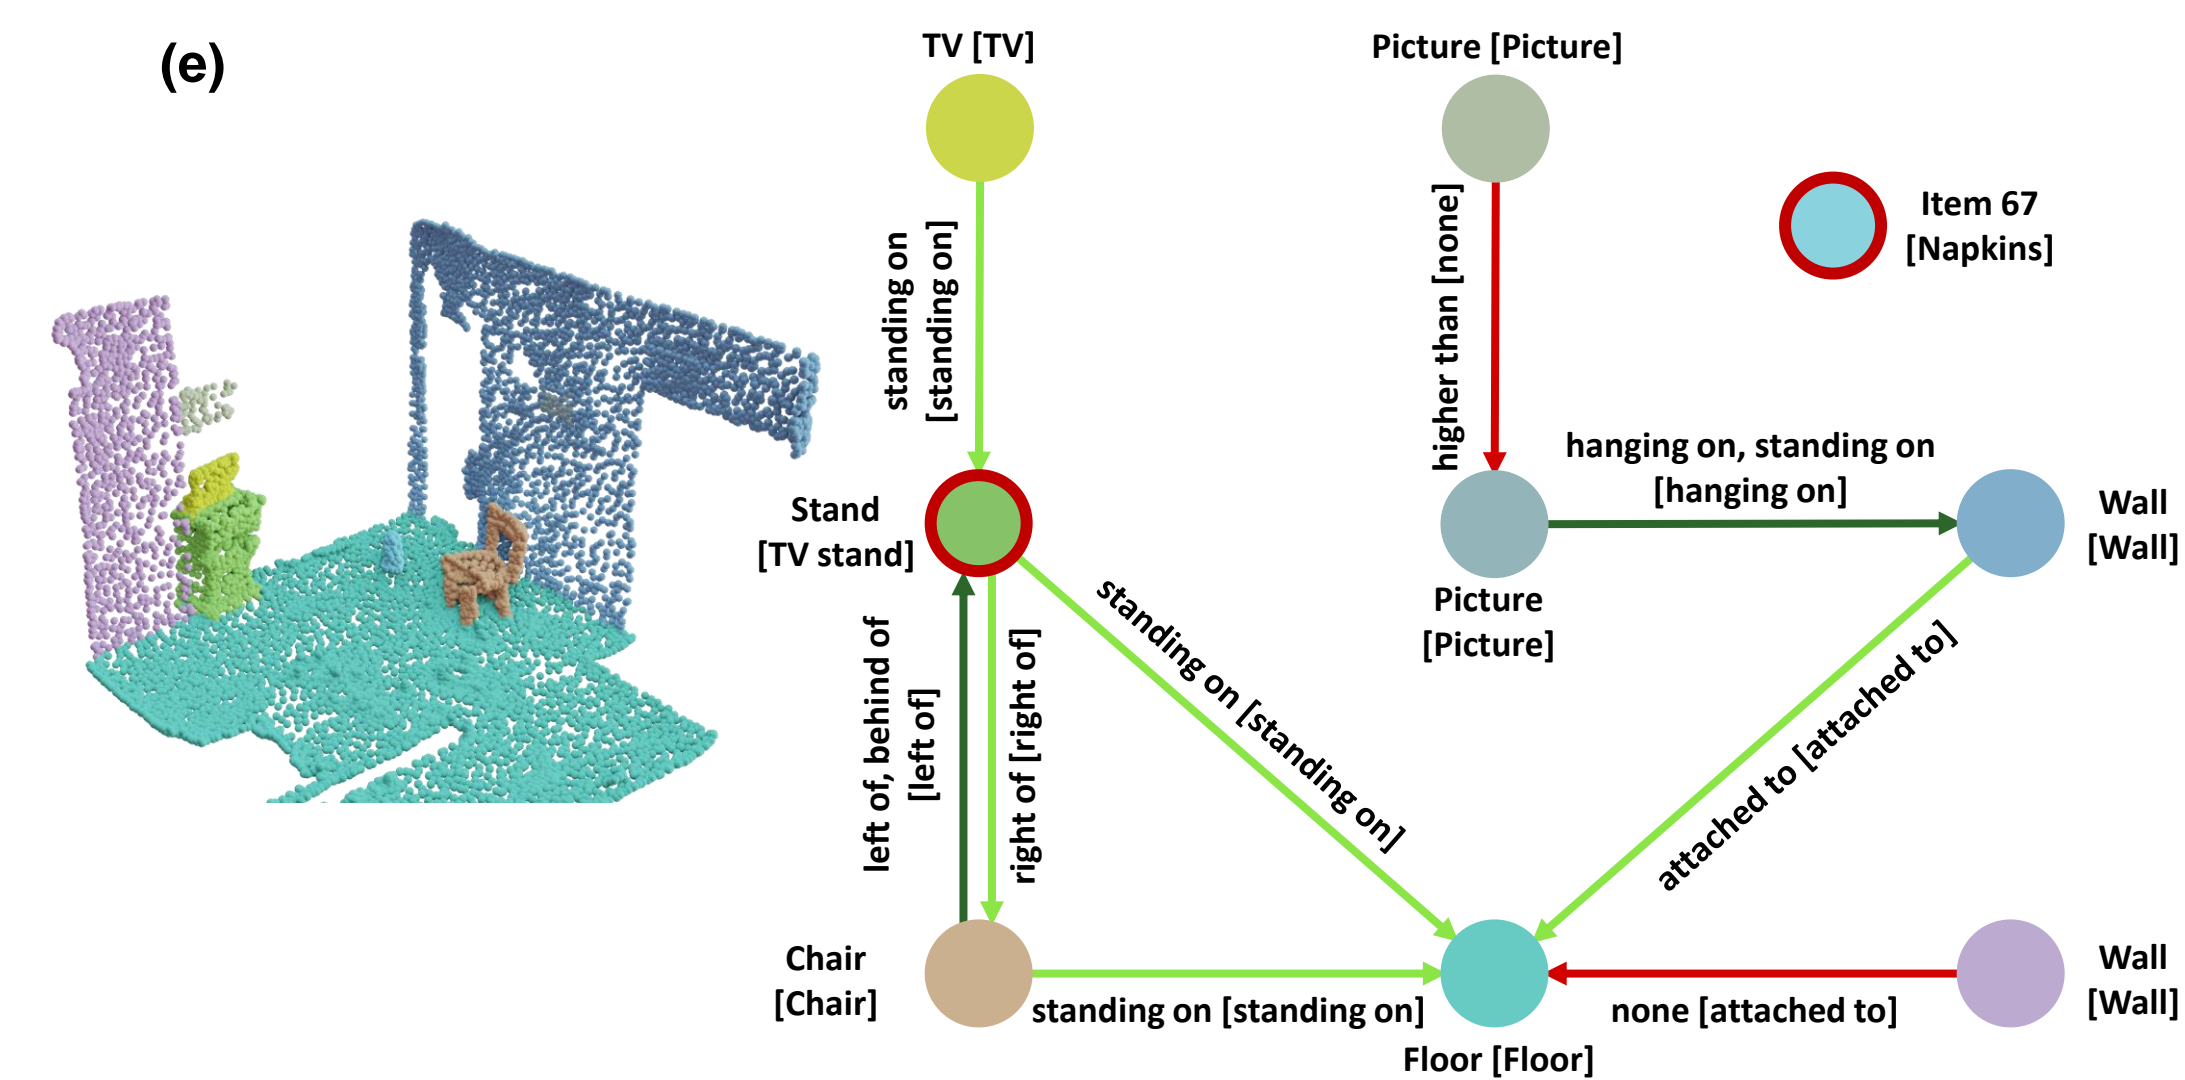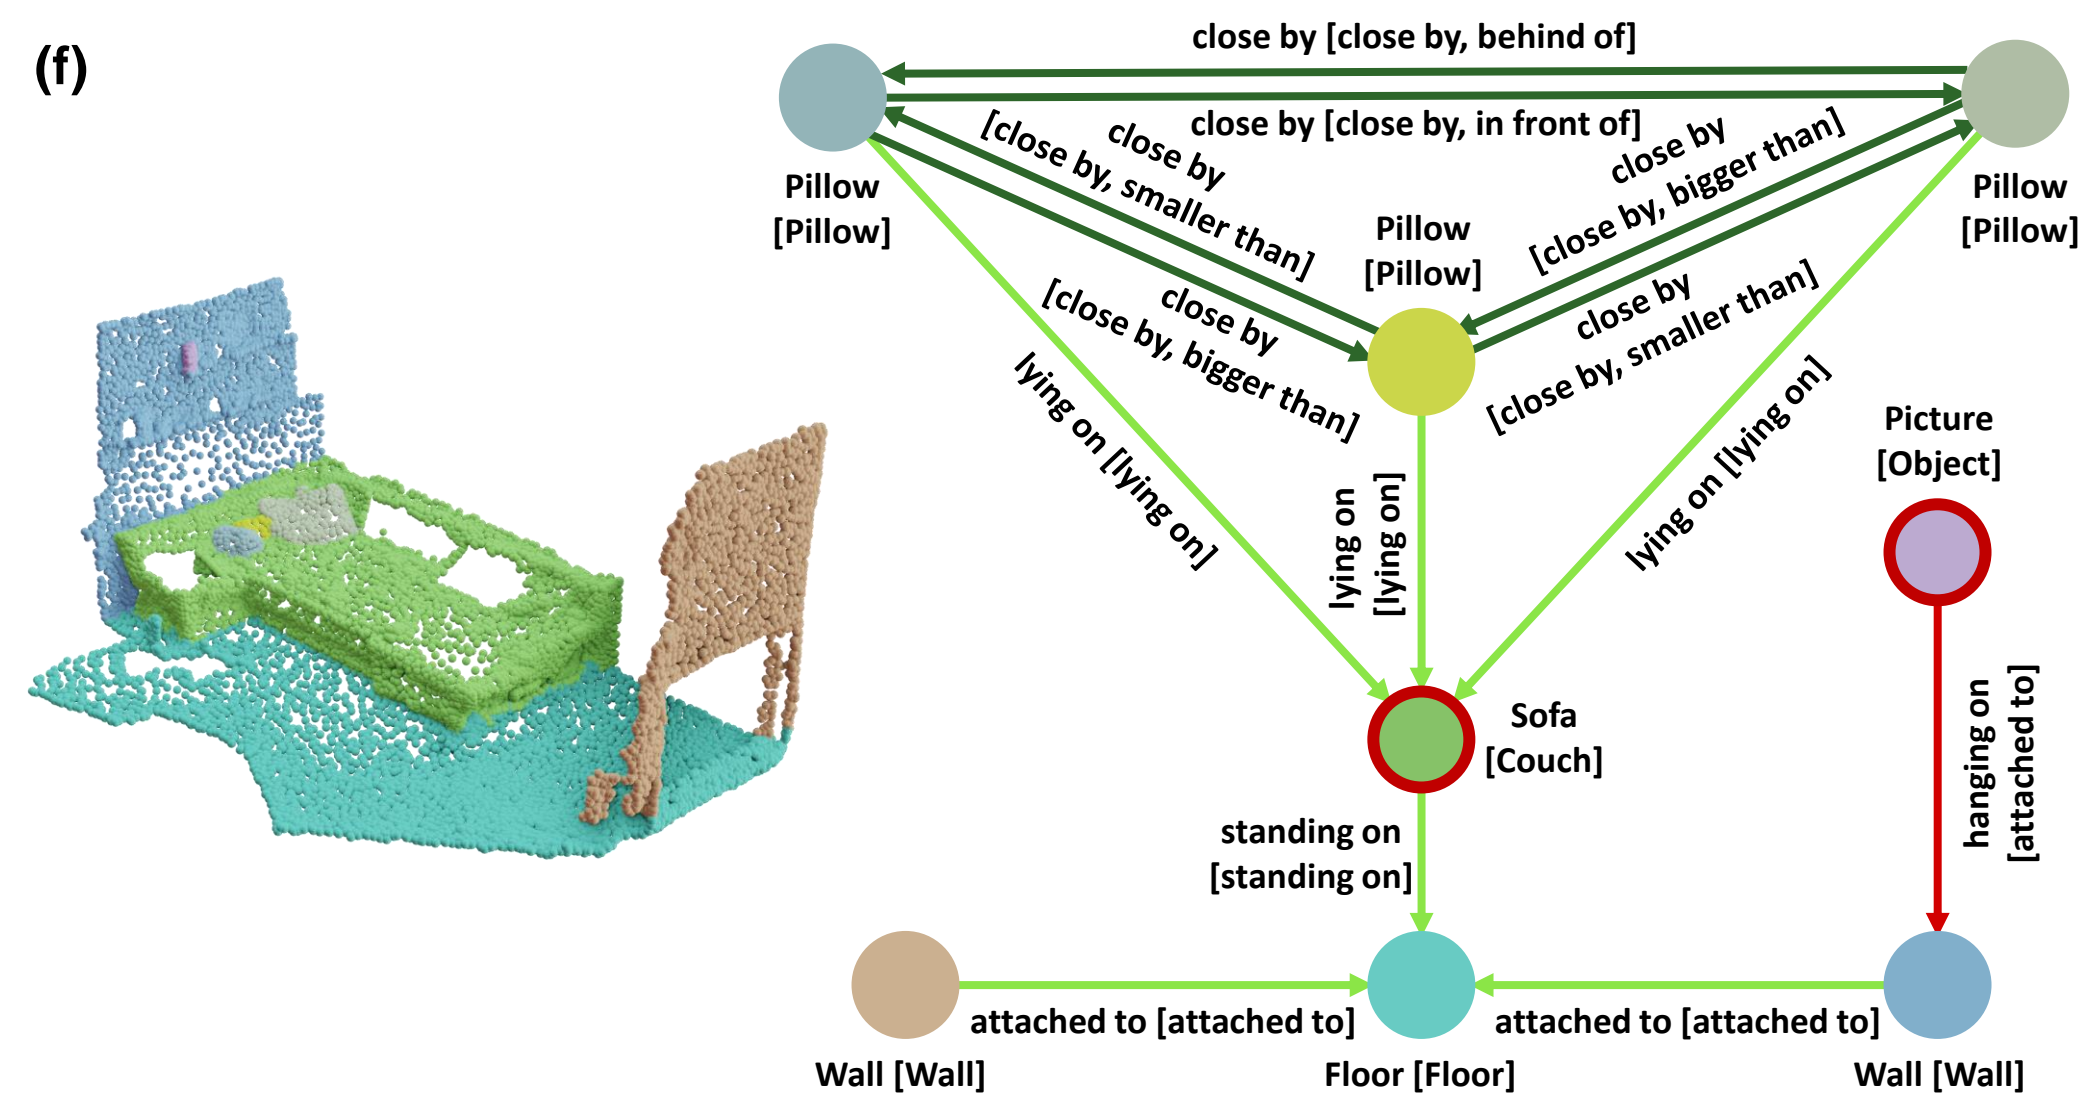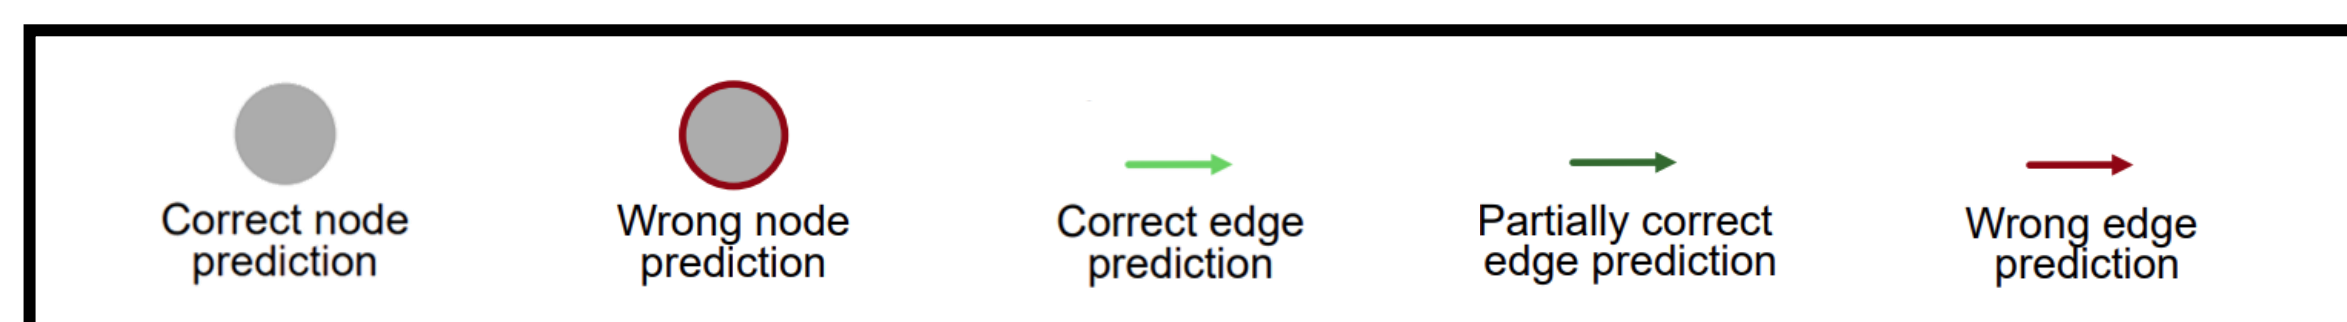



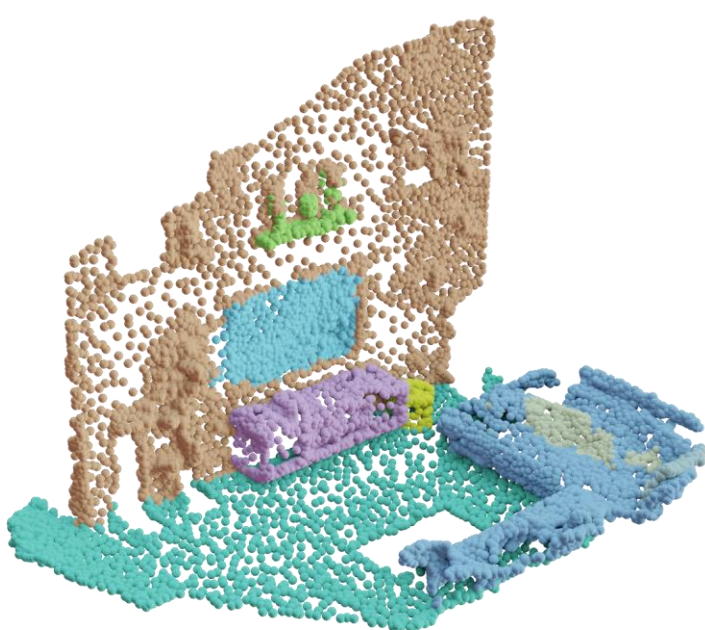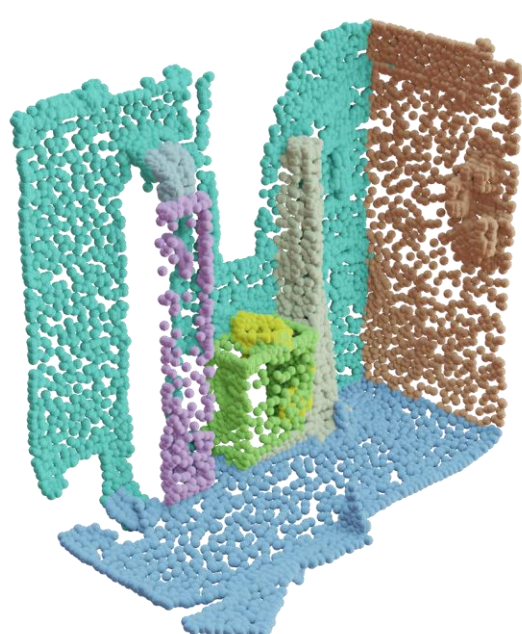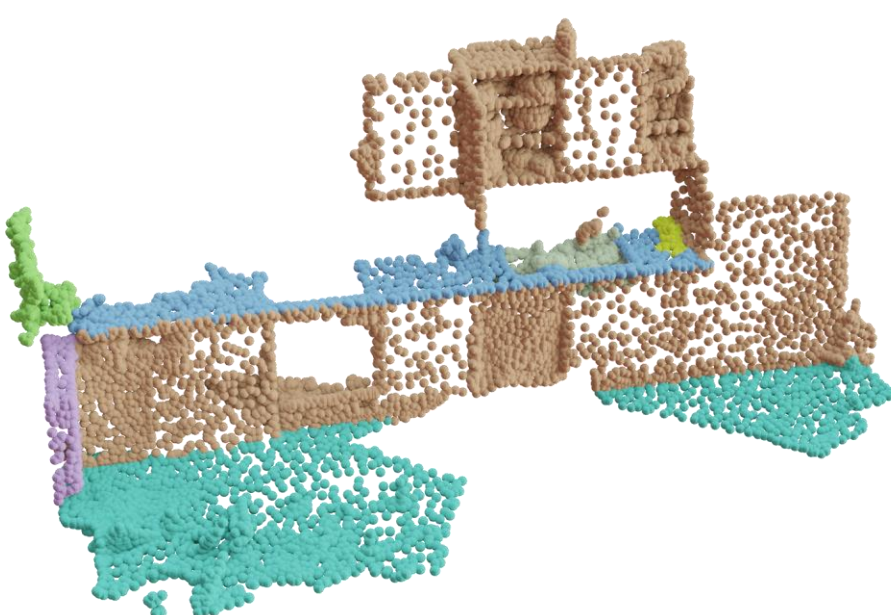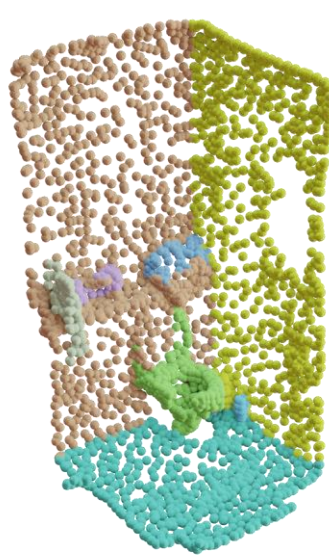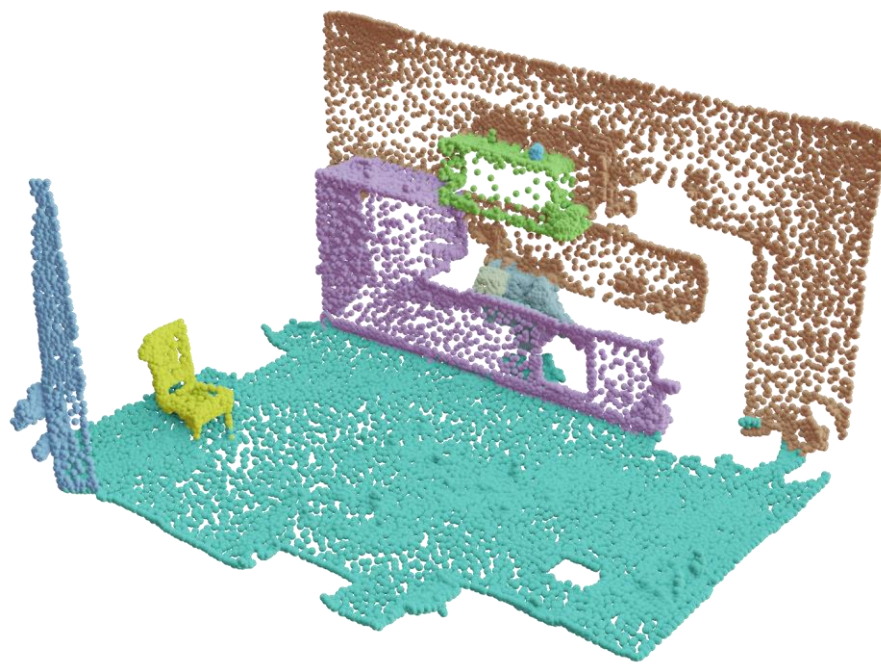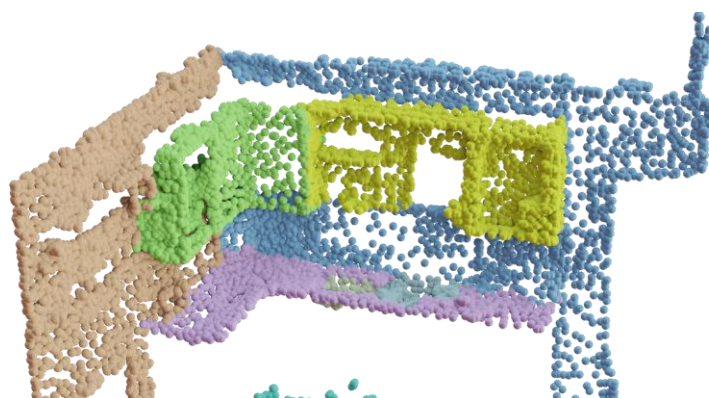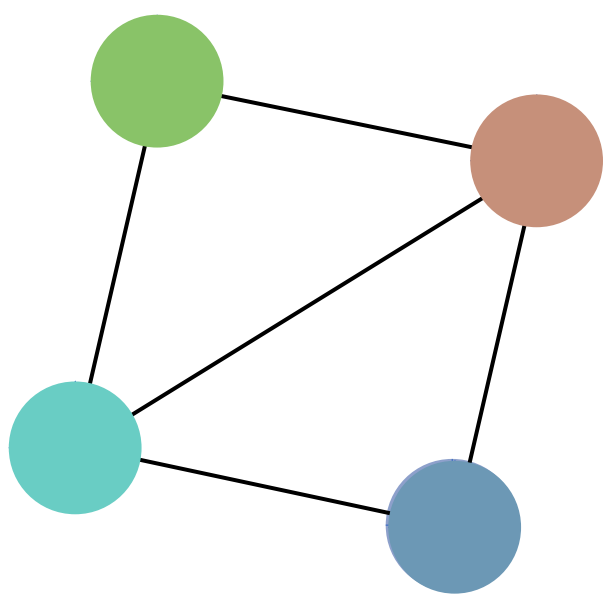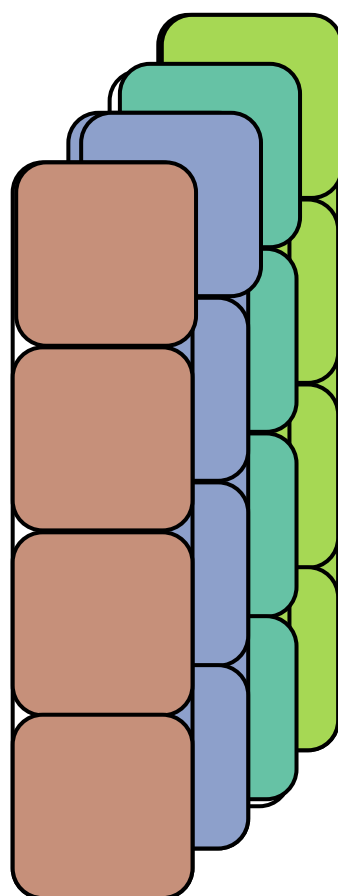

Supplement: Supplementary file 1 [file supp.pdf]
